# Supplementary material for: Multipartite quantum synchronization in driven-dissipative spin networks
Source: arXiv:2606.24360 source file (2026-10-10)
Supplement: Supplementary file 1 [file Supplementry.tex]

\documentclass[aps,prl,reprint]{revtex4-2}

\usepackage{amsmath,amssymb,graphicx,bm}
\usepackage[colorlinks=true,citecolor=blue]{hyperref}

\begin{document}

\title{Supplemental Material for:
``Multipartite synchronization residuals in driven-dissipative spin networks''}

\author{Jatin Ghildiyal}
\email{jatin.20phz0017@iitrpr.ac.in} % Replace with the actual email
\author{Shubhrangshu Dasgupta}
\author{Asoka Biswas}
\affiliation{Department of Physics, Indian Institute of Technology Ropar, Rupnagar, Punjab 140001, India}

\maketitle

\section{Hamiltonian of two qubits}

We investigate the subadditivity of synchronization in a system of two spatially separated qubits that interact indirectly through photon tunneling between two coupled cavities. Each qubit is locally coupled to its respective cavity mode via a Jaynes-Cummings interaction, while coherent hopping between the cavity modes mediates an effective qubit-qubit interaction (Fig. 1 in the main text). Such cavity-assisted coupling provides a flexible platform for exploring collective dynamics and synchronization phenomena in open quantum systems.
The Hamiltonian of the system is
\begin{equation}
\begin{aligned}
H &=
\sum_{i=1}^{2}\Big[
\omega_c a_i^\dagger a_i
+ \frac{1}{2}\omega_i\sigma_z^{(i)}
+ g_i (a_i + a_i^\dagger)(\sigma_+^{(i)} + \sigma_-^{(i)})
\\
&\quad+ \varepsilon_c \big(a_i e^{-i\omega_d t} + a_i^\dagger e^{i\omega_d t}\big)
+ \frac{1}{2}\varepsilon_q\big(\sigma_+^{(i)} e^{-i\omega_q t}
+ \sigma_-^{(i)} e^{i\omega_q t}\big)
\Big] \\
&\quad
+ \sum_{\langle i,j\rangle} J_{ij}
\left(a_i^\dagger a_j + a_j^\dagger a_i\right).
\end{aligned}
\end{equation}
Here $a_i$ ($a_i^\dagger$) annihilates (creates) a photon in cavity $i$ of frequency $\omega_c$, and $\sigma_z^{(i)},\sigma_\pm^{(i)}$ denote Pauli operators for qubit $i$ with transition frequency $\omega_i$. The parameter $g_i$ is the qubit–cavity coupling strength, $J_{ij}$ is the photon hopping amplitude between cavities, and $\varepsilon_c$ and $\varepsilon_q$ specify coherent drives at frequencies $\omega_d$ and $\omega_q$, respectively.
Under the rotating-wave approximation, rapidly oscillating counter-rotating contributions are neglected, yielding the effective driven Hamiltonian
\begin{equation}
\begin{aligned}
H_{\mathrm{RWA}} &=
\sum_{i=1}^{2}\Big[
\Delta_c a_i^{\dagger} a_i
+ \frac{1}{2}\Delta_i\sigma_z^{(i)}
+ g_i \left(a_i^{\dagger} \sigma_-^{(i)} + \sigma_+^{(i)} a_i \right)\\
&\quad
+ \frac{1}{2}\varepsilon_q\sigma_x^{(i)}
+ \varepsilon_c (a_i + a_i^{\dagger})
\Big]
+ \sum_{\langle i,j\rangle} J_{ij}
\left(a_i^{\dagger} a_j + a_j^{\dagger} a_i \right).
\end{aligned}
\end{equation}
In the parameter regime where the cavity modes evolve on a timescale much shorter than that of the qubits, the photonic degrees of freedom may be adiabatically eliminated. We then obtain the following effective two-qubit Hamiltonian in the dispersive regime ($\Delta_c \gg \Delta_i,g_i$):
\begin{small}
\begin{equation}
\begin{aligned}
H &= \sum_{i=1}^{2}\Bigg[
\frac{1}{2}\left(\Delta_i - \frac{\Delta_c g_i^2}{\Delta_c^2 - J_{12}^2}\right)\sigma_z^{(i)}
+ \frac{1}{2}\left(\varepsilon_q - \frac{2 g_i \varepsilon_c}{\Delta_c + J_{12}}\right)\sigma_x^{(i)}
\Bigg]\\&\quad
+ \frac{g_1 g_2 J_{12}}{\Delta_c^2 - J_{12}^2}
\left(\sigma_+^{(1)}\sigma_-^{(2)}+\mathrm{h.c.}\right).
\label{hamiladia}
\end{aligned}
\end{equation}
\end{small}

\section{Hamiltonian of three qubits}
Assuming the cavity modes can be adiabatically eliminated (i.e. cavity detuning and hopping set the fastest timescale compared to the qubit dynamics), we obtain an effective Hamiltonian for the reduced qubit manifold, starting from Eq. (14) in the main paper with $n=3$. In compact, general form the Hamiltonian is
\begin{widetext}
\begin{equation}
\begin{aligned}
H
&=
\sum_{i=1}^{3}
\Bigg[
\frac{\Delta_i}{2}\sigma_z^{(i)}
+
\frac{\varepsilon_q}{2}\sigma_x^{(i)}
+
\frac{1}{Y}
\Big(
g_i\!\left[AX^{\dagger}(i)\sigma_-^{(i)}+\sigma_+^{(i)}AX(i)\right]
+
\varepsilon_c\!\left[AX(i)+AX^{\dagger}(i)\right]
\Big)
\Bigg]
\\
&\quad
+
\frac{1}{Y^{2}}\Bigg[
\sum_{i=1}^{3}
\left[
\Delta_c\,AX^{\dagger}(i)AX(i)
\right]
+
\sum_{\substack{i=1 \\ i \neq j}}^3 J_{ij}
\left[
AX^{\dagger}(i)AX(j)+AX^{\dagger}(j)AX(i)
\right]\Bigg]\;,
\end{aligned}
\label{hamil3}
\end{equation}
\end{widetext}
where $Y= \Delta_c^3 - \Delta_c\bigl(J_{12}^2 + J_{23}^2 + J_{31}^2\bigr) + 2\,J_{12}J_{23}J_{31}$ and the operators
$
X(i)\equiv \varepsilon_c+g_j\sigma_-^{(i)}
$
combine the local drive and qubit-assisted excitation channels. The geometry of the mediated interactions is encoded in the symmetric matrix
\[
A =
\begin{pmatrix}
J_{23}^2 - \Delta_c^2 & J_{12}\Delta_c - J_{23}J_{31} & J_{31}\Delta_c - J_{12}J_{23} \\
J_{12}\Delta_c - J_{23}J_{31} & J_{31}^2 - \Delta_c^2 & J_{23}\Delta_c - J_{12}J_{31} \\
J_{31}\Delta_c - J_{12}J_{23} & J_{23}\Delta_c - J_{12}J_{31} & J_{12}^2 - \Delta_c^2
\end{pmatrix},
\]
whose elements depend on the intercavity hopping amplitudes and the cavity detuning. This matrix determines both the magnitude and sign of the effective couplings and therefore specifies how the triangular photonic network mediates correlations among the qubits. The resulting Hamiltonian (\ref{hamil3}) has been used in solving the Lindblad equation for three qubits. 

\section{Derivation of bipartite synchronization residual}
To construct a collective synchronization measure, we represent the
joint distribution $P_{12}(\phi_1,\phi_2)$ in terms of  the relative phase coordinate
$\phi_{-}^{(12)} \;\equiv\; (\phi_1 - \phi_2)/2 \;\in\; (-\pi,\, \pi)$. 
Therefore, the marginal
distributions take the following form:
\begin{eqnarray}
P_{12}(\phi_{-}^{(12)})
&=&
\int_0^{2\pi}
P_{12}(\phi_{1},\phi_2)\,
d\phi_+^{(12)},
\label{eq:P12_proj}
\end{eqnarray}
where $\phi_+^{(12)}=(\phi_1+\phi_2)/2$.
Since $P_{12}(\phi_1,\phi_2)$ is positive definite and is normalized over
$[0,2\pi)$, the marginals $P_{j}(\phi_j)$ and $P_{12}(\phi_-^{(12)})$ are non-negative and normalized.

It is convenient to decompose the phase distributions into a uniform background $1/2\pi$ and a fluctuation term $D_j(\phi_j)$, i.e., $P_j(\phi_j)=\frac{1}{2\pi}+D_j(\phi_j)$,
where the fluctuation integrates to zero, i.e., $\int_0^{2\pi} D_j(\phi_j)\, d\phi_j =0.$
Substituting this decomposition into Eq.~(4) in the main text, we get
\begin{equation}
R_j=\left|\int_0^{2\pi}D_j(\phi_j)\,e^{i\phi_j}\, d\phi_j\right|.
\end{equation}
Further, from the Eq. (5) in the main text, we obtain
\begin{small}
\begin{equation}
\begin{aligned}
P_{12}(\phi_1,\phi_2)
&=
\left(
\frac{1}{2\pi}
+
D_1(\phi_1)
\right)
\left(
\frac{1}{2\pi}
+
D_2(\phi_2)
\right)
+
C_{12}(\phi_1,\phi_2)
\\
&=
\frac{1}{(2\pi)^2}
+
\frac{1}{2\pi}D_1(\phi_1)
+
\frac{1}{2\pi}D_2(\phi_2)
\\
&\quad
+
D_1(\phi_1)D_2(\phi_2)
+
C_{12}(\phi_1,\phi_2).
\end{aligned}
\label{B2}
\end{equation}
\end{small}
Integrating (\ref{B2}) with respect to the variable $\phi_+^{(12)}$, we project the above expression onto the space of the relative phase coordinate $\phi_-^{(12)}$ via
Eq.~\eqref{eq:P12_proj} to obtain the following equation:
\begin{equation}
\begin{aligned}
D_{12}(\phi_{-}^{(12)})
&=
\frac{1}{2\pi}D_1(\phi_{-}^{(12)})
+
\frac{1}{2\pi}D_2(\phi_{-}^{(12)})\\&\quad
+
\left[D_1 D_2\right]_{(\phi_{-}^{(12)})}
+ C_{12}(\phi_{-}^{(12)}),
\label{eq:D12_exact}
\end{aligned}
\end{equation}
where we have used $P_{12}(\phi_-^{(12)})=(\tfrac{1}{2\pi})^2+D_{12}(\phi_-^{(12)})$ and
\begin{equation}
D_j(\phi_{-}^{(12)}) = \int_{0}^{2\pi}D_j(\phi_j)d\phi_{+}^{(12)}\;, \;\;\;j\in \{1,2\}\;.
\end{equation}

Here $[D_1 D_2]_{\phi_-^{(12)}}$ denotes the projection of the nonlinear product term
onto the $\phi_{-}^{(12)}$- space, as given by
\begin{equation}
\left[D_1 D_2\right]_{(\phi_{-}^{(12)})}
\equiv
\int_0^{2\pi} D_1(\phi_{1})\,D_2(\phi_2)\,d\phi_{+}^{(12)},
\end{equation}
and 
\begin{equation}
C_{12}(\phi_{-}^{(12)}) \equiv \int_0^{2\pi}
C_{12}(\phi_1,\phi_2)\,d\phi_+^{(12)}
\label{deltac}
\end{equation}
is the projection of the
correlation function. Both projected terms satisfy the zero-mean condition
$\int_{-\pi}^{\pi}[\cdots]\,d\phi_{-}^{(12)}=0$ by linearity of the projection and the
marginal constraints on $D_j$ and $C_{12}$.
The functions $R_{j}$ are defined through the modulus of the
first moment of $D_{j}(\phi_{-}^{(12)})$. Defining the first  moment of a function $f(\phi_{-}^{(12)})$ as
\begin{equation}
\mathcal{F}[f]
\equiv
\int_{-\pi}^{\pi} f(\phi_{-}^{(12)})\, e^{i\phi_{-}^{(12)}}\, d\phi_{-}^{(12)},
\end{equation}
we obtain from the Eq.~\eqref{eq:D12_exact} gives
\begin{equation}
\mathcal{F}[D_{12}]
=
\frac{1}{2\pi}\mathcal{F}[D_1]
+
\frac{1}{2\pi}\mathcal{F}[D_2]
+
\mathcal{F}\!\left[\left[D_1 D_2\right]_{\phi_{-}^{(12)}}\right]
+
\mathcal{F}[\delta C_{12}].
\end{equation}
Taking the absolute value on both sides, we get
\begin{equation}
R_{12}
=
\left|\,
\frac{1}{2\pi}\mathcal{F}[D_1]
+
\frac{1}{2\pi}\mathcal{F}[D_2]
+
\mathcal{F}[\delta{C}_{12}]
\,\right|,
\end{equation}
where 
\begin{equation}
\delta{C}_{12}(\phi_{-}^{(12)})
\equiv
\left[D_1 D_2\right]_{\phi_{-}^{(12)}} +  C_{12}(\phi_{-}^{(12)}).
\end{equation}

Applying the triangle inequality and using $1/(2\pi) < 1$, we obtain
\begin{equation}
R_{12}
\le
\frac{1}{2\pi}\left|\mathcal{F}[D_1]\right|
+
\frac{1}{2\pi}\left|\mathcal{F}[D_2]\right|
+
\left|\mathcal{F}[\delta{C}_{12}]\right|
\le
R_1
+
R_2
+
R_C,
\end{equation}
where
\begin{equation}
R_C
=
\left|
\int_{-\pi}^{\pi}
\delta{C}_{12}(\phi_{-}^{(12)})\,
e^{i\phi_{-}^{(12)}}\, d\phi_{-}^{(12)}
\right|
\end{equation}
quantifies the contribution of inter-subsystem correlations to phase coherence.

The condition $R_C = 0$ holds whenever the combined correlation term
$\delta{C}_{12}(\phi_{-}^{(12)})$ carries no first harmonic. This is
satisfied in the physically important case where the two subsystems are
statistically independent, so $C_{12}\equiv 0$, and the nonlinear product
$[D_1 D_2]_{\phi_{-}^{(12)}}$ has zero projection onto $e^{i\phi_{-}^{(12)}}$. 
More generally,
$R_C = 0$ holds whenever inter-subsystem correlations and nonlinear mixing
effects do not contribute to the mean-field order parameter.

The synchronization measure then satisfies
\begin{equation}
R_{12}(t)
\le
R_1(t)
+
R_2(t)\;, \;\;\Delta_R^{(2)}\ge 0.
\end{equation}
This relation bounds the
collective phase coherence by the sum of the local synchronization measures and
therefore constrains the maximum synchronization that can be generated at the
bipartite level.

\section{Derivation of tripartite synchronization residual}
We start with Eq. (11) in the main text which after integration with respect to $\phi_2$ leads to
\begin{small}
\begin{align}
&D_{123}(\phi_-^{(12)},\phi_-^{(23)})
=
\frac{1}{2\pi}
\int_0^{2\pi}
D_1(2\phi_-^{(12)}+\phi_2)D_2(\phi_2)\,d\phi_2\nonumber\\
&+\frac{1}{2\pi}
\int_0^{2\pi}
D_1(2\phi_-^{(12)}+\phi_2)D_3(\phi_2-2\phi_-^{(23)})\,d\phi_2
\nonumber\\
&
+\frac{1}{2\pi}
\int_0^{2\pi}
D_2(\phi_2)D_3(\phi_2-2\phi_-^{(23)})\,d\phi_2\nonumber\\
&+\int_0^{2\pi}
D_1(2\phi_-^{(12)}+\phi_2)D_2(\phi_2)D_3(\phi_2-2\phi_-^{(23)})\,d\phi_2\nonumber\\
&+C_{13}(\phi_-^{(12)},\phi_-^{(23)})+\Gamma_{13;2}(\phi_-^{(12)},\phi_-^{(23)}) \nonumber\\
&+C_{123}{(\phi_-^{(12)},\phi_-^{(23)})}\;,
\label{eq:P1P2P3}
\end{align}
\end{small}
where we have used $P_{123}(\phi_-^{(12)},\phi_-^{(23)})=\frac{1}{(2\pi)^2}+D_{123}(\phi_-^{(12)},\phi_-^{(23)})$. Here, the terms linear in $D_j$ vanish upon integration over $\phi_2$ because of mean-field condition, i.e.,
\begin{equation}
\int_0^{2\pi}D_1(2\phi_-^{(12)}+\phi_2)\,d\phi_2=0,
\quad
\int_0^{2\pi}D_3(\phi_2-2\phi_-^{(23)})\,d\phi_2=0.
\end{equation}
Here
\begin{align}
2\pi C_{13}(\phi_-^{(12)},\phi_-^{(23)}) &=
\int_0^{2\pi}
C_{13}(2\phi_-^{(12)}+\phi_2,\phi_2-2\phi_-^{(23)})
\,d\phi_2\;,\nonumber\\
\Gamma_{13;2}(\phi_-^{(12)},\phi_-^{(23)})
&=
\int_0^{2\pi}
C_{13}(2\phi_-^{(12)}+\phi_2,\phi_2-2\phi_-^{(23)})
\nonumber\\
&\qquad\times
D_2(\phi_2)\,d\phi_2\;,\nonumber\\
C_{123}
(\phi_-^{(12)},\phi_-^{(23)})
&=
\int_0^{2\pi}
C_{123}
(2\phi_-^{(12)}+\phi_2,\phi_2,
\phi_2-2\phi_-^{(23)})
\,d\phi_2\;.
\end{align}

The bipartite synchronization measure associated with a pair of subsystems is
\begin{eqnarray}
{R}_{ij}
&=
\left|
\int_{-\pi}^{\pi}
P_{ij}(\phi_-^{(ij)})
e^{i\phi_-^{(ij)}}
\,d\phi_-^{(ij)}
\right|\nonumber\\
&=\left|
\int_{-\pi}^{\pi}
D_{ij}(\phi_-^{(ij)})
e^{i\phi_-^{(ij)}}
\,d\phi_-^{(ij)}
\right|.
\end{eqnarray}
Similarly, the three-body synchronization measure can be obtained from the tripartite phase distribution as 
\begin{align}
{R}_{123}&=\left|\int_{-\pi}^{\pi}P_{123}(\Phi_-)e^{i\Phi_-}\,d\Phi_-
\right|\nonumber\\
&=\left|\int_{-\pi}^{\pi}D_{123}(\Phi_-)e^{i\Phi_-}\,d\Phi_-
\right|,
\label{R123}
\end{align}
where 
\begin{align}
P_{123}(\Phi_-)&=\int_{-\pi}^{\pi}P_{123}(\phi_-^{(12)},\phi_-^{(23)})d\Phi_+\;,\nonumber\\
    D_{123}(\Phi_-)&=\int_{-\pi}^{\pi}D_{123}(\phi_-^{(12)},\phi_-^{(23)})d\Phi_+\;,
    \label{P123}
\end{align}
and $\Phi_{\pm} = (\phi_-^{(12)}\pm \phi_-^{(23)})/2$.

To obtain an inequality involving the $R$-functions, we next introduce the conditional distribution
\begin{equation}
P_{12|23}(\phi_-^{(12)}|\phi_-^{(23)})
=
\frac{P_{123}(\phi_-^{(12)},\phi_-^{(23)})}
{P_{23}(\phi_-^{(23)})},
\end{equation}
where 
\begin{equation}
    P_{23}(\phi_-^{(23)})=\int_0^{2\pi}P_{23}(\phi_2,\phi_3)d\phi^{(23)}_{+}
\end{equation}
with $\phi^{(23)}_{+}=(\phi_2+\phi_3)/2$.

The above expression of tripartite phase distribution can be rewritten as

\begin{align}
R_{123}
&=
\left|
\int_{-\pi}^{\pi}\int_{-\pi}^{\pi}
P_{123}\!\left(\phi_-^{(12)},\phi_-^{(23)}\right)
e^{i\Phi_-}
\,d\Phi_+\,d\Phi_-
\right|
\nonumber\\[2mm]
&=
\Biggl|
\int_{-\pi}^{\pi}
P_{23}\!\left(\phi_-^{(23)}\right)
e^{-i\phi_-^{(23)}}
\nonumber\\
&\qquad\times
\Biggl[
\int_{-\pi}^{\pi}
P_{12|23}\!\left(
\phi_-^{(12)}\big|\phi_-^{(23)}
\right)
e^{i\phi_-^{(12)}}
\,d\phi_-^{(12)}
\Biggr]
\,d\phi_-^{(23)}
\Biggr|.
\end{align}
Note that the change in integration variables $\Phi_\pm \rightarrow \{\phi_-^{(12)},\phi_-^{(23)}\}$ involves a Jacobian which is unity. 

Defining
\begin{equation}
{R}_{12|23}(\phi_-^{(23)})
=
\left|
\int_{-\pi}^\pi
P_{12|23}(\phi_-^{(12)}|\phi_-^{(23)})
e^{i\phi_-^{(12)}}
d\phi_-^{(12)}
\right|,
\end{equation}
we obtain using 
the triangle inequality
\begin{equation}
{R}_{123}
\le
\int_{-\pi}^{\pi}
P_{23}(\phi_-^{(23)})
{R}_{12|23}(\phi_-^{(23)})
\,d\phi_-^{(23)}.
\label{eq:bound1}
\end{equation}

Adding and subtracting ${R}_{12}$ inside the integral and using
the normalization of $P_{23}$ yields
\begin{align}
{R}_{123}
\le
{R}_{12}
+
\int_{-\pi}^{\pi}
P_{23}(\phi_-^{(23)})
\Big[
{R}_{12|23}(\phi_-^{(23)})
-
{R}_{12}
\Big]
d\phi_-^{(23)}.
\label{eq:main}
\end{align}
The integrand above can be interpreted as the enhancement in the phase synchronization between subsystems 1 and 2, conditioned on the phase synchronization between subsystems 2 and 3. However, this additional synchronization cannot exceed the synchronization resource already available between subsystems 2 and 3, beyond that available in subsystem 2 alone. This means that if subsystems 1 and 2 are synchronized between themselves, any enhancement of their synchronization is possible due to their coupling to subsystem 3, if subsystems 2 and 3 are themselves synchronized. We therefore can introduce an upper bound to (\ref{eq:main}), as

\begin{equation}
\int_{-\pi}^{\pi}
P_{23}(\phi_-^{(23)})
\Big[
{R}_{12|23}(\phi_-^{(23)})
-
{R}_{12}
\Big]
d\phi_-^{(23)}
\le
{R}_{23}
-
{R}_{2}.
\label{eq:corr}
\end{equation}

Substituting Eq.~(\ref{eq:corr}) into Eq.~(\ref{eq:main}), we finally obtain
\begin{equation}
{R}_{123}(t)
+
{R}_{2}(t)
\le
{R}_{12}(t)
+
{R}_{23}(t)\;,\;\;\Delta_R^{(3)}\ge 0\;,
\label{eq:SSA}
\end{equation}
which constitutes the SSA-like relation for the
synchronization measure. Equality is attained when the conditioning on
$\phi_-^{(23)}$ supplies exactly the maximal admissible coherence, which corresponds to a 
joint distribution factorized as 
\begin{equation}
P_{123}(\phi_-^{(12)},\phi_-^{(23)})
=
\frac{
P_{12}(\phi_-^{(12)})
P_{23}(\phi_-^{(23)})
}{
P_2(\phi_2)
}.
\end{equation}
This refers to the absence of genuine three-body correlations,
$C_{123}^{(3)}\equiv0$.

The inequality (\ref{eq:SSA}) shows that the collective synchronization shared among the three subsystems, together with the contribution of the intermediate subsystem, cannot exceed the sum of the two bipartite synchronization channels. The structure is therefore directly analogous to the strong subadditivity property of quantum entropy.

We emphasize that the violation of the inequality (\ref{eq:SSA}) can be essentially attributed to our usage of Husimi-Q function in obtaining the phase distribution functions. This Q functions represents a quasi-probability function, instead of a true probability function and therefore the violation occurs.

\end{document}
